# Supplementary material for: Controlling the microstructure and phase behavior of confined soft colloids by active interaction switching
Source: arXiv:2004.04566 ancillary file (2020-04-09)
Supplement: Supplementary file 1 [file SUPPLEMENTAL_MATERIAL.pdf]

# Controlling the microstructure and phase behavior of confined colloids by active interaction switching

## SUPPLEMENTAL MATERIAL

### A. Time evolution of a homogeneous mixture of switching particles

In this section we investigate the time evolution of the particle concentrations for an homogeneous mixture (bulk) in which species b and s can be switched

$$\mathrm{b} \rightleftharpoons \mathrm{s} \qquad \text{(A-1)}$$

We consider the binary system formed by $N_\mathrm{b}$ particles of type 'b' and $N_\mathrm{s}$ particles of type 's' contained inside a volume $V$. The bulk number densities of both species are $\rho_i = N_i/V$ ($i$ = b, s). The total number density is $\rho_\mathrm{T} = \rho_\mathrm{b} + \rho_\mathrm{s}$, and the composition parameter is defined as $x = \rho_\mathrm{s}/\rho_\mathrm{T}$. Particles of type b are converted into s at a rate $k_\mathrm{bs}$, whereas particles of type s convert into b at a rate $k_\mathrm{sb}$, following this set of coupled kinetic reaction equations:

$$\left.\begin{aligned} \frac{d\rho_\mathrm{b}}{dt} &= k_\mathrm{sb}\rho_\mathrm{s} - k_\mathrm{bs}\rho_\mathrm{b} \\ \frac{d\rho_\mathrm{s}}{dt} &= k_\mathrm{bs}\rho_\mathrm{b} - k_\mathrm{sb}\rho_\mathrm{s} \end{aligned}\right\}$$

(A-2)

The first term of the right hand represents the production, whereas the second one the disappearance of this component. These coupled differential equations are analytically solvable, starting from the initial conditions $\rho_\mathrm{b}(t=0) = \rho_\mathrm{b0}$ and $\rho_\mathrm{s}(t=0) = \rho_\mathrm{s0}$, leading to the following time dependent concentrations

$$\begin{aligned} \rho_\mathrm{b}(t) &= \frac{1}{k_\mathrm{bs}+k_\mathrm{sb}}\left[\left(\rho_\mathrm{b0}k_\mathrm{bs} - \rho_\mathrm{s0}k_\mathrm{sb}\right)e^{-(k_\mathrm{bs}+k_\mathrm{sb})t} + k_\mathrm{sb}\rho_\mathrm{T0}\right] \\ \rho_\mathrm{s}(t) &= \frac{1}{k_\mathrm{bs}+k_\mathrm{sb}}\left[\left(\rho_\mathrm{s0}k_\mathrm{sb} - \rho_\mathrm{b0}k_\mathrm{bs}\right)e^{-(k_\mathrm{bs}+k_\mathrm{sb})t} + k_\mathrm{bs}\rho_\mathrm{T0}\right] \end{aligned} \qquad \text{(A-3)}$$

where $\rho_\mathrm{T0} = \rho_\mathrm{b0} + \rho_\mathrm{s0}$.

**Figure SM-1** illustrates the time evolution of the concentrations provided by Eq. (A-3) for the particular case of $\rho_\mathrm{b0} = 2$, $\rho_\mathrm{s0} = 1$, $k_\mathrm{bs} = 4$ and $k_\mathrm{sb} = 1$ (arbitrary units). As observed, both concentrations vary exponentially with time at the same rate to finally reach asymptotically the final equilibrium state, in which the concentrations become constant.

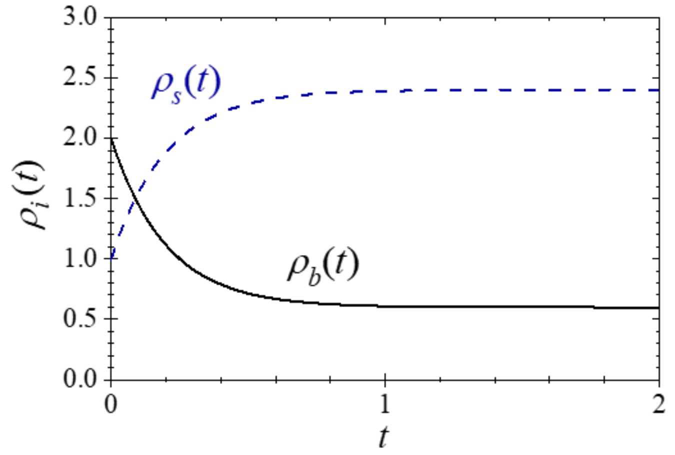


**Figure SM-1**: Time evolution of the concentrations of species b and s for $\rho_{b0} = 2$, $\rho_{s0} = 1$, $k_{bs} = 4$ and $k_{sb} = 1$ (arbitrary units).

During the whole process, the total number of particles remains invariable, i.e. in terms of concentrations $\rho_b(t) + \rho_s(t) = \rho_{b0} + \rho_{s0}$, but the relative composition changes. The final equilibrium concentrations are given by

$$\rho_{b,\infty} = \lim_{t\to\infty} \rho_b(t) = \frac{k_{sb}}{k_{bs} + k_{sb}} \rho_{T0}$$
$$\rho_{s,\infty} = \lim_{t\to\infty} \rho_s(t) = \frac{k_{bs}}{k_{bs} + k_{sb}} \rho_{T0} \tag{A-3}$$

In particular, if the initial composition $x_0$ is chosen to fulfill the condition

$$\frac{x_0}{1 - x_0} = \frac{\rho_{s0}}{\rho_{b0}} = \frac{k_{bs}}{k_{sb}} \tag{A-4}$$

then the system is originally in equilibrium at $t = 0$ and the integration of the kinetic equations A-2 leads to a time-independent solution, namely $\rho_b(t) = \rho_{b0}$ and $\rho_s(t) = \rho_{s0}$.

**B. Integration of the active reaction-diffusion equations provided by reaction dynamical density functional theory (R-DDFT)**

The R-DDFT framework leads to the following coupled equations of the number densities of big and small colloids in the presence of **switching activity**:

$$\frac{\partial \rho_{\mathrm{b}}(\mathbf{r},t)}{\partial t} = -\nabla\cdot\mathbf{J}_{\mathrm{b}} + k_{\mathrm{sb}}\rho_{\mathrm{s}}(\mathbf{r},t) - k_{\mathrm{bs}}\rho_{\mathrm{b}}(\mathbf{r},t)$$
$$\frac{\partial \rho_{s}(\mathbf{r},t)}{\partial t} = -\nabla\cdot\mathbf{J}_{s} + k_{\mathrm{bs}}\rho_{\mathrm{b}}(\mathbf{r},t) - k_{\mathrm{sb}}\rho_{\mathrm{s}}(\mathbf{r},t) \quad \text{(B-1)}$$

The diffusive fluxes are given by

$$\mathbf{J}_{i} = -D_{i}\rho_{i}(\mathbf{r},t)\nabla\left[\beta\mu_{i}(\mathbf{r},t)\right] \quad \text{(B-2)}$$

where

$$\beta\mu_{i}(\mathbf{r},t) = \frac{\delta\beta F}{\delta\rho_{i}(\mathbf{r},t)} \quad \text{(B-3)}$$

is the functional derivative of the **total** system free energy, but replacing the equilibrium density profiles by the time-dependent nonequilibrium profiles $\rho_i(\mathbf{r},t)$. As both kinetic rate constants are connected to preserve the bulk concentrations, we can use one of them, for instance $k_{\mathrm{bs}}$, to characterize the switching rate. $k_{\mathrm{bs}}$ can be written as the inverse of the characteristic big-to-small conversion time, $k_{\mathrm{bs}} = 1/\tau$. This time can be compared to the typical diffusion time for small particles, given by $\tau_0 = \sigma_{\mathrm{s}}^2/D_{\mathrm{s}}$. The switching activity is defined as

$$a = \frac{\tau_0}{\tau} \quad \text{(B-4)}$$

The task of finding out the correct free energy for a mixture of colloids can be in general very challenging. Fortunately, Gaussian pair potentials

$$\beta u_{ij}(r) = \varepsilon_{ij} e^{-r^2/\sigma_{ij}^2} \qquad i, j = \mathrm{b}, \mathrm{s} \quad \text{(B-5)}$$

are soft, and it has been shown that this system behaves as a weakly correlated mean-field fluid over a surprisingly wide density and temperature range, being more accurate as the particle densities increase [Louis *et al.*, Phys. Rev. E **62**, 7961 (2000)]**.** In the presence of external potentials acting on the big and small particles, the mean-field free energy functional can be decomposed into three additive contributions: ideal, excess and external free energy terms:

$$\beta F\left[\{\rho_i(\mathbf{r},t)\}\right]=\beta F_{\text{id}}\left[\{\rho_i(\mathbf{r},t)\}\right]+\beta F_{\text{ex}}\left[\{\rho_i(\mathbf{r},t)\}\right]+\beta F_{\text{ext}}\left[\{\rho_i(\mathbf{r},t)\}\right]=$$

$$\begin{aligned}&=\sum_{i=\text{b,s}}\int\rho_i(\mathbf{r},t)\left[\ln(\rho_i(\mathbf{r},t)\Lambda_i^3)-1\right]d\mathbf{r}\\&+\frac{1}{2}\sum_{i=\text{b,s}}\int\int\rho_i(\mathbf{r},t)\rho_j(\mathbf{r}',t)\beta u_{ij}(|\mathbf{r}-\mathbf{r}'|)d\mathbf{r}d\mathbf{r}'\\&+\sum_{i=\text{b,s}}\int\beta u_i^{\text{ext}}(\mathbf{r})\rho_i(\mathbf{r},t)d\mathbf{r}\end{aligned} \qquad \text{(B-6)}$$

where $\Lambda_I = h/(2\pi m k_B T)^{1/2}$ ($i$ = b, s) are the thermal wave lengths of both species, and $\rho_i(\mathbf{r},t)$ are the space-dependent density profiles induced by the external potentials $u_i^{\text{ext}}(\mathbf{r})$, which makes the particle concentrations inhomogeneous. The resulting inhomogeneous chemical potential are given by

$$\beta\mu_i(\mathbf{r},t)=\frac{\delta\beta F}{\delta\rho_i(\mathbf{r})}=\ln(\rho_i(\mathbf{r},t)\Lambda_i^{3})+\beta u_i^{\text{ext}}(\mathbf{r})+\underbrace{\sum_{j=b.s}\int\rho_j(\mathbf{r},t)\beta u_{ij}(|\mathbf{r}-\mathbf{r}'|)d\mathbf{r}'}_{\beta\mu_i^{\text{ex}}(\mathbf{r},t)} \qquad \text{(B-7)}$$

So

$$\mathbf{J}_i=-D_i\rho_i(\mathbf{r},t)\nabla\left[\beta\mu_i(\mathbf{r},t)\right]=-D_i\left[\nabla\rho_i(\mathbf{r},t)+\rho_i(\mathbf{r},t)\nabla\beta\left(u_i^{\text{ext}}(\mathbf{r})+\mu_i^{\text{ex}}(\mathbf{r},t)\right)\right] \qquad \text{(B-8)}$$

This mean-field approximation is equivalent to the so-called random phase approximation (RPA) for the direct correlation function, obtained from the second functional derivative of the excess free energy (in equilibrium)

$$c_{ij}(|\mathbf{r}-\mathbf{r}'|)=-\frac{\delta^2 F_{\text{ex}}}{\delta\rho_i(\mathbf{r})\delta\rho_j(\mathbf{r}')}=-\beta u_{ij}(|\mathbf{r}-\mathbf{r}'|) \qquad \text{(B-9)}$$

It is important to remark here that if the external potentials $u_i^{\text{ext}}(\mathbf{r})$ are time independent, then switching activity does not produce time-oscillating density profiles or another kind of unsteady regimes. In all cases, the system evolves in time until a steady state is eventually reached. However, this final (activity-induced) state does not imply that the net fluxes are zero, as occur under non-active equilibrium conditions. Instead, the steady-state density profiles in the presence of switching activity are the solution to

$$\begin{aligned}\nabla\cdot\mathbf{J}_{\text{b}}&=k_{\text{sb}}\rho_{\text{s}}(\mathbf{r},t)-k_{\text{bs}}\rho_{\text{b}}(\mathbf{r},t)\\\nabla\cdot\mathbf{J}_s&=k_{\text{bs}}\rho_b(\mathbf{r},t)-k_{\text{sb}}\rho_s(\mathbf{r},t)\end{aligned} \qquad \text{(B-10)}$$

so the **net diffusive fluxes are balanced by the production and disappearance of particles** due to the switching activity.

In the main text of the manuscript, we make use of the R-DDFT method (Eqs. B1, B2 and B3) to determine the non-equilibrium concentrations of active system in the presence of two representative non-homogeneous situations: mixtures near a planar hard wall and phase separated mixtures confined inside a spherical cavity. For mixtures close to the planar wall, the density profiles depend only on the distance to the wall, *z*, so

$$\nabla\cdot\mathbf{J}_i = \frac{\partial J_i}{\partial z} \qquad J_i(z) = -D_i\rho_i(z,t)\frac{\partial\beta\mu_i}{\partial z} \qquad \text{(planar symmetry)} \qquad \text{(B-11)}$$

For particles confined in the spherical cavity, the density profiles have spherical symmetry, so the equations depend on the distance to the center of the cavity, $r$. In this case

$$\nabla\cdot\mathbf{J}_i = \frac{1}{r^2}\frac{\partial}{\partial r}\left(r^2 J_i\right) \qquad J_i(r) = -D_i\rho_i(r,t)\frac{\partial\beta\mu_i}{\partial r} \qquad \text{(spherical symmetry)} \quad \text{(B-12)}$$

In order to solve Eqs. B1-B3 three boundary conditions must be specified:

**Condition 1** regards the knowledge of the initial density profiles, $\rho_i(\mathbf{r},0) = \rho_{i0}(\mathbf{r})$.

**Conditions 2** and **3** involve the value of the particle densities at two different locations, which may vary depending of the specific situation under consideration. For mixtures close to a **planar hard wall**, these conditions are:

**Condition 2**: $\rho_i(z\to\infty,t) = \rho_i^{\text{bulk}}$ (homogeneous fluid far from the wall).

**Condition 3**: $J_i(z=0,t) = 0$ (zero net fluxes at the impenetrable wall).

For mixtures confined inside a **spherical cavity** of radius $R$, we have:

**Condition 2**: $J_i(r=R,t) = 0$ (zero net fluxes at the confining spherical wall)

**Condition 3**: $J_i(r=0,t) = 0$ (zero net fluxes at the center of the cavity due to spherical symmetry)

In order to numerically integrate the R-DDFT equations we use a spatial grid of $\Delta z = \Delta r = 0.01\sigma_s$. The time step has been fixed to $\Delta t/\tau_0 = 2.5\cdot 10^{-5}$, which is small enough to avoid the appearance of numerical instabilities ($\Delta t < \Delta z^2/(2D_s)$). For the case of mixtures near a single hard wall, the integration extends over a distance of $z_{max} = 20\sigma_s$. This distance is large enough to avoid undesired finite-size effects. The particle concentrations in constant to the wall were determined with high degree of accuracy extrapolating the values in the limit of $\Delta z \to 0$.

## C. Time-dependent non-equilibrium density profiles of active mixtures close to a planar wall

We here show the time-dependent nonequilibrium density profiles of system S1 (see Table I in the main text of the manuscript) near a planar hard wall induced by the presence of switching activity $a = 1$. For this purpose, we start at time $t = 0$ from the equilibrium profiles corresponding to a non-active equilibrium system ($a = 0$), and turn on the activity at $t > 0$. **Figure SM-2** shows the time evolution of the normalized density profiles of big (top panel) and small (bottom panel), obtained solving the R-DDFT equations with planar symmetry. The initial equilibrium density profiles are shown as gray squares.

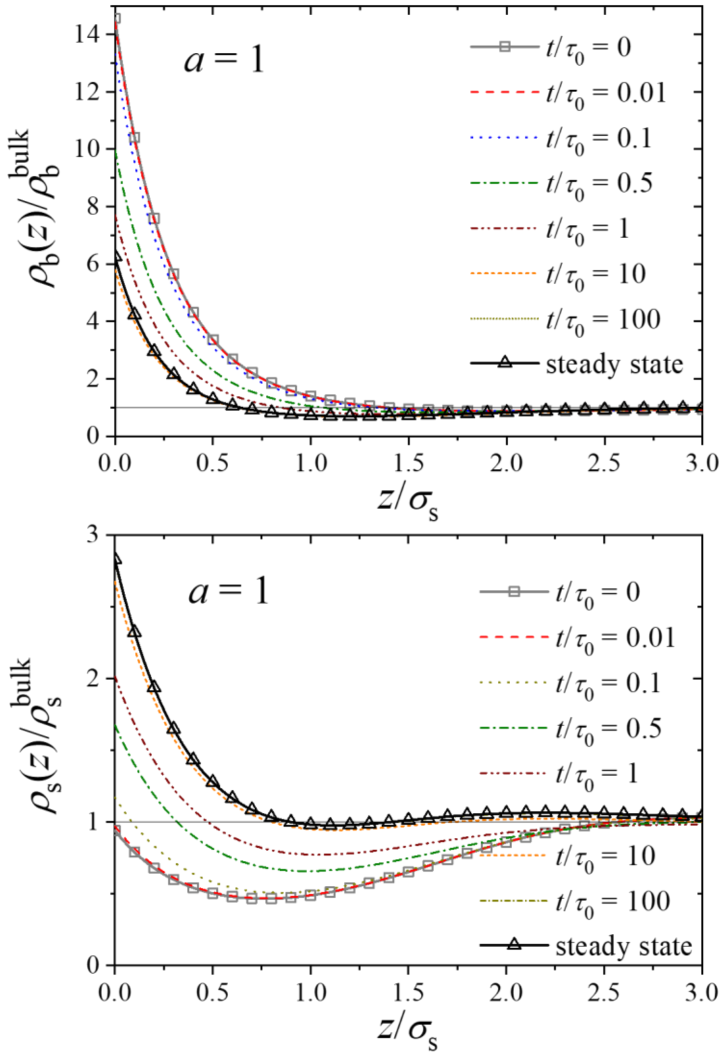


**Figure SM-2**: Time evolution of the density profiles of big (top panel) and small (bottom panel) particles near a hard wall (system S1). For $t = 0$ the profiles correspond to the equilibrium state without activity. For $t > 0$, the exchange activity $a = 1$ is turned on, which triggers the evolution of the density profiles to the new steady state.

The local densities evolve rapidly at short times and finally converge to the new steady state in which the effect of the activity is exactly balanced by the flux rates according to Eqs. B-9 (black triangles in Figure SM-2). As observed, activity induces a profound modification of the density profiles near the wall, even though the bulk concentrations remain unaltered. The adsorption peak of big particles decreases whereas the concentration of small particles close to the wall shows an important increase coupled with a reduction of the depletion region.

## D. Time evolution of phased separated active mixtures confined inside a spherical cavity

In this section of the Supplemental Material we show the time-dependent nonequilibrium density profiles of system S3 in a spherical cell. This particular choice of interaction parameters and particle concentrations correspond to a system located inside the unstable region of the phase diagram. Therefore, system S3 undergoes spontaneous demixing in equilibrium. We confine the mixture inside a spherical cavity of radius $R = 5\sigma_{\rm s}$, using the following confining potential:

$$\beta u_i^{\rm ext}(r) = \begin{cases} 10(r/R)^{10} & r \le R \\ \infty & r > R \end{cases} \qquad i = {\rm b,s} \tag{D.1}$$

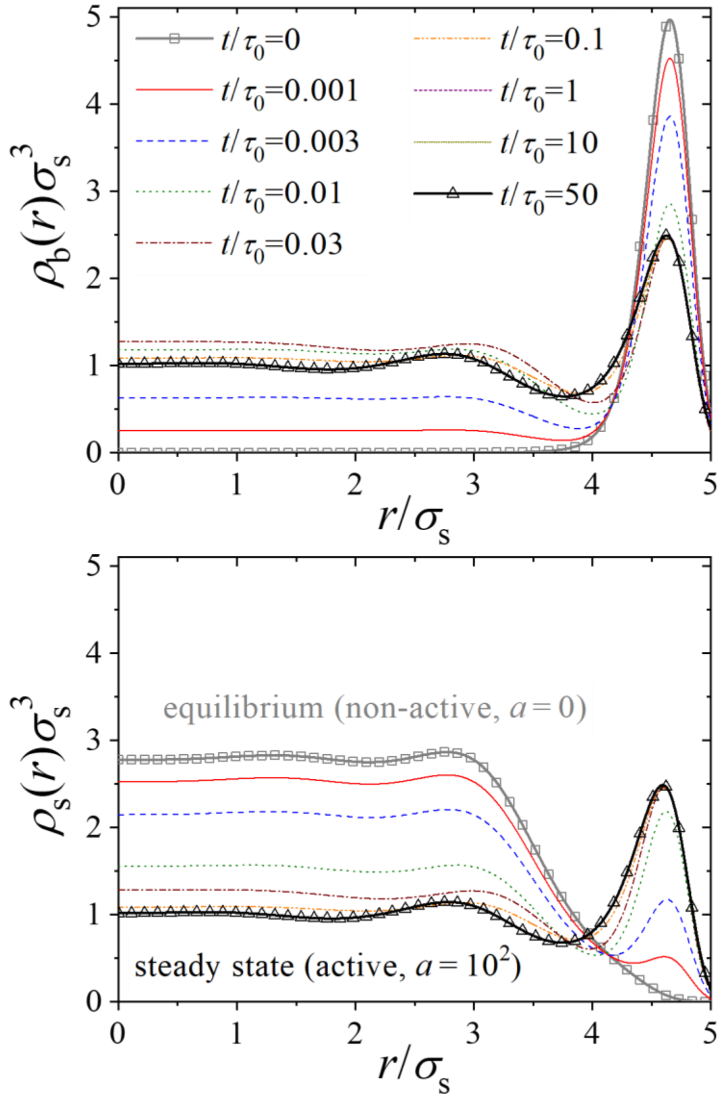


**Figure SM-3**: Time evolution of the density profile of big (top panel) and small (bottom panel) particles confined inside a spherical cavity (system S3). For $t = 0$ are in the demixed equilibrium state corresponding to the non-active case. For $t > 0$, the exchange activity $a = 10^2$ is turned on, which triggers the evolution of the density profiles up to the new steady state.

**Figure SM-3** shows the time evolution of the normalized density profiles of big (top panel) and small (bottom panel), obtained solving the R-DDFT equations in a spherical compartment.

In a first step, we integrate the R-DDFT equations with spherical symmetry for a nonactive system ($a = 0$) to obtain a phase separated mixture inside the cavity. For this purpose, we start the calculation assuming a homogeneous mixture of both components, and let the system evolve until the system converges to the equilibrium distribution. Gray lines with square symbols in both graphs of Figure SM-3 represent the final equilibrium one-body density profiles. It is evident that, in equilibrium the system exhibits spontaneous fluid-fluid demixing in the cavity. Indeed, big particles are mostly adsorbed close to the outer wall of the cavity (please note the large peak located at $r \approx 4.7\sigma_s$) whereas small ones are mainly distributed in the central region of the cavity. This particular segregation of particles in the demixed system is not a whimsical effect, but is a well-known physical phenomenon observed in wetting transitions. In fact, the accumulation of larger particles into a narrow layer near the wall is caused by the existence of an effective attraction between the outer wall and the larger component. This effect arises because the repulsion induced by the wall, $u_i^{\text{ext}}(r)$, even though is the same for both species, has a longer range on the scale of the small particles. This effect leads to an enhanced depletion of small spheres close to the wall, which in turn induces an effective attraction of the big component to the wall [Archer and Evans, J. Phys.: Condens. Matter **14**. 1131 (2002)].

In a second step, we solve the R-DDFT equations to calculate the time evolution of the density profiles in the presence of switching activity. Again, we initiate the calculations at $t = 0$ taking the phase-separated density profiles corresponding to a non-active system ($a = 0$) as initial state, and turning on the activity $a = 10^2$ at $t > 0$. Colored lines of Figure SM-3 depict the time evolution of density profiles of the big and small Gaussian particles. As observed, as time increases, the height of the main peak of $\rho_b(r)$ decreases whereas the concentration in the central region shows a non-monotonic behavior, as it increases for $t/\tau_0 < 0.03$, and then decreases until it finally reaches the steady state regime for $t/\tau_0 < 0.03$, represented by black lines with up-triangles. We interpret this behavior as a transient rearrangement of the big particles induced by the strong and fast reduction of the main peak. $\rho_s(r)$ shows the opposite trend: the initial large concentration of small particles in the center of the cavity decreases as time progresses, and a peak is formed close to the wall of the spherical cavity. In this case, the value of the activity ($a = 10^2$) is so large that both profiles converge to a common shape, inducing a complete mixing of the phase-separated system, as discussed in the main text of the manuscript.
